# Supplementary material for: The metallicity effect on line-depth ratios in APOGEE $H$-band spectra
Source: arXiv:1901.07141 ancillary file (2019-01-22)

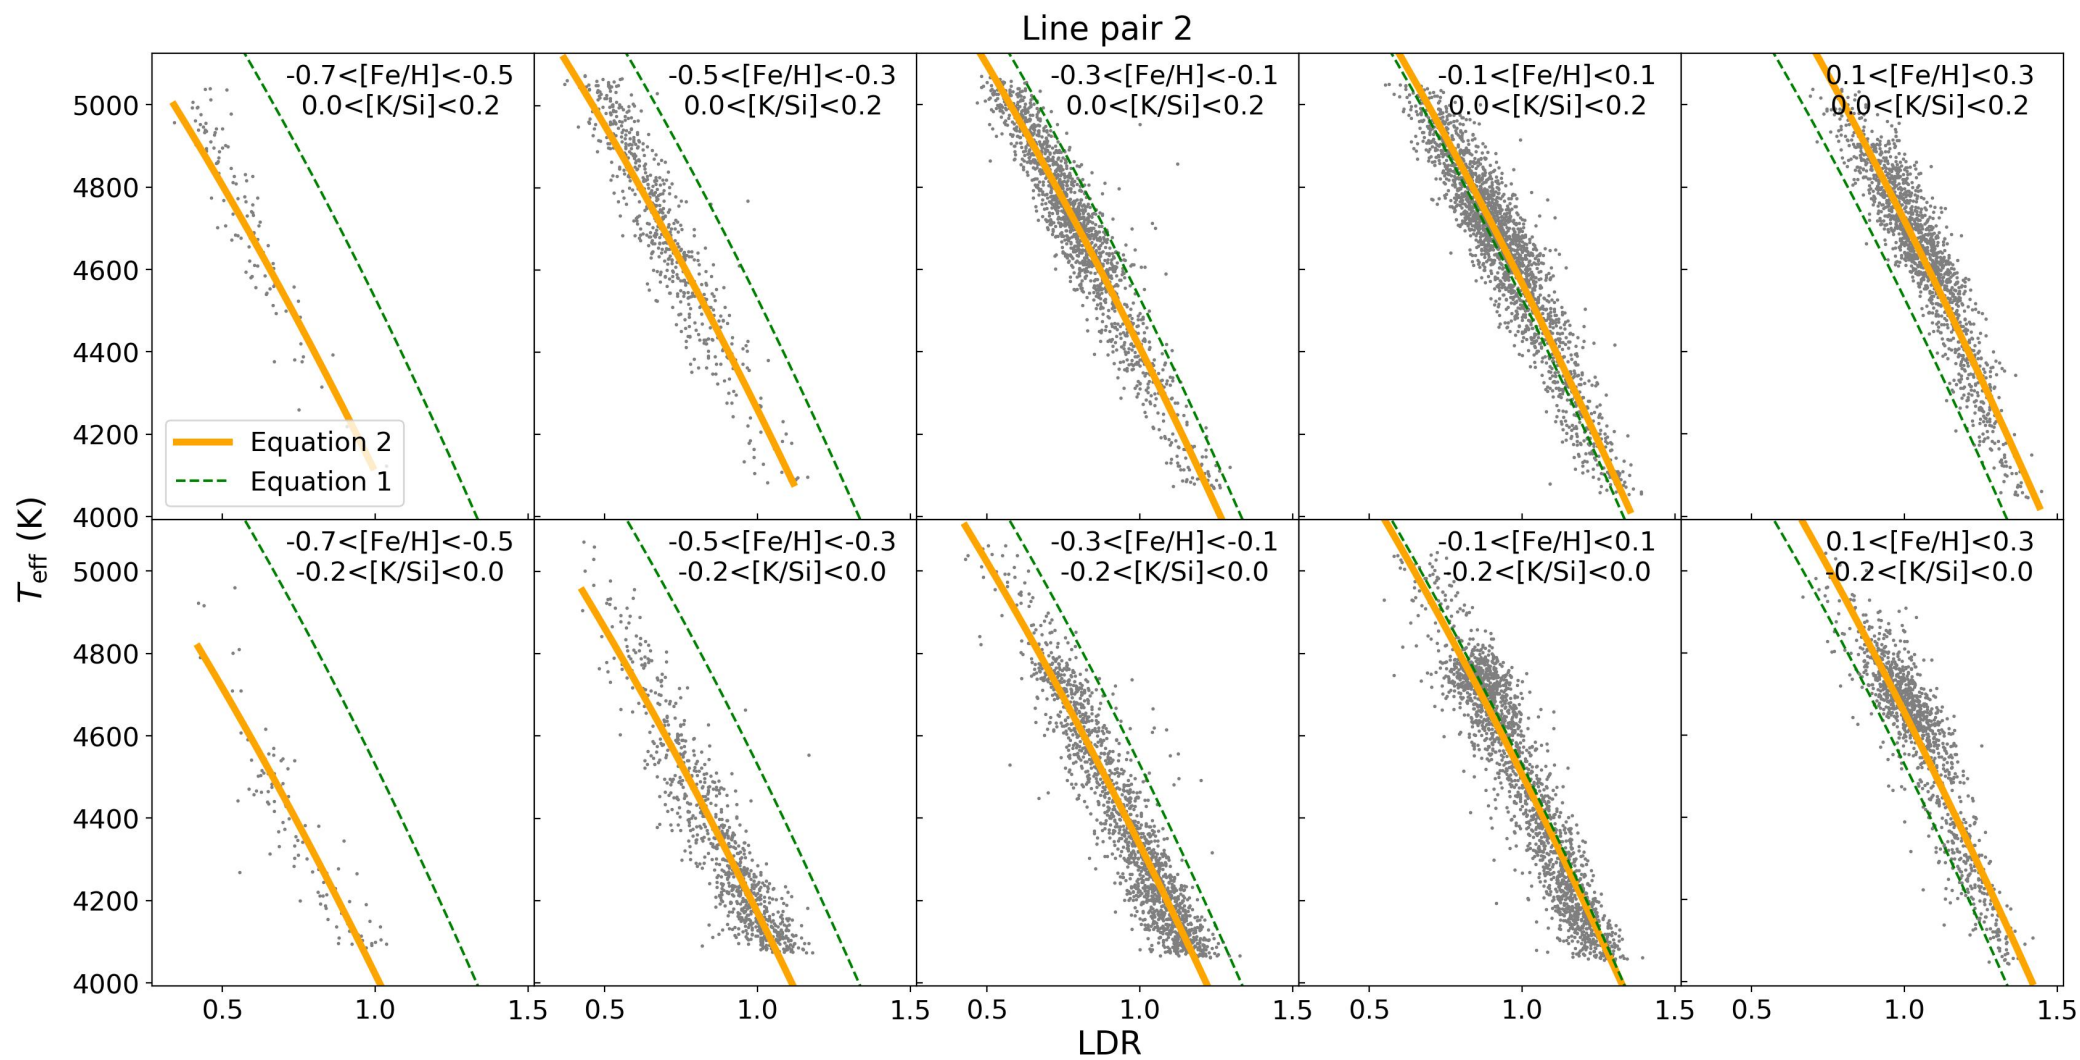

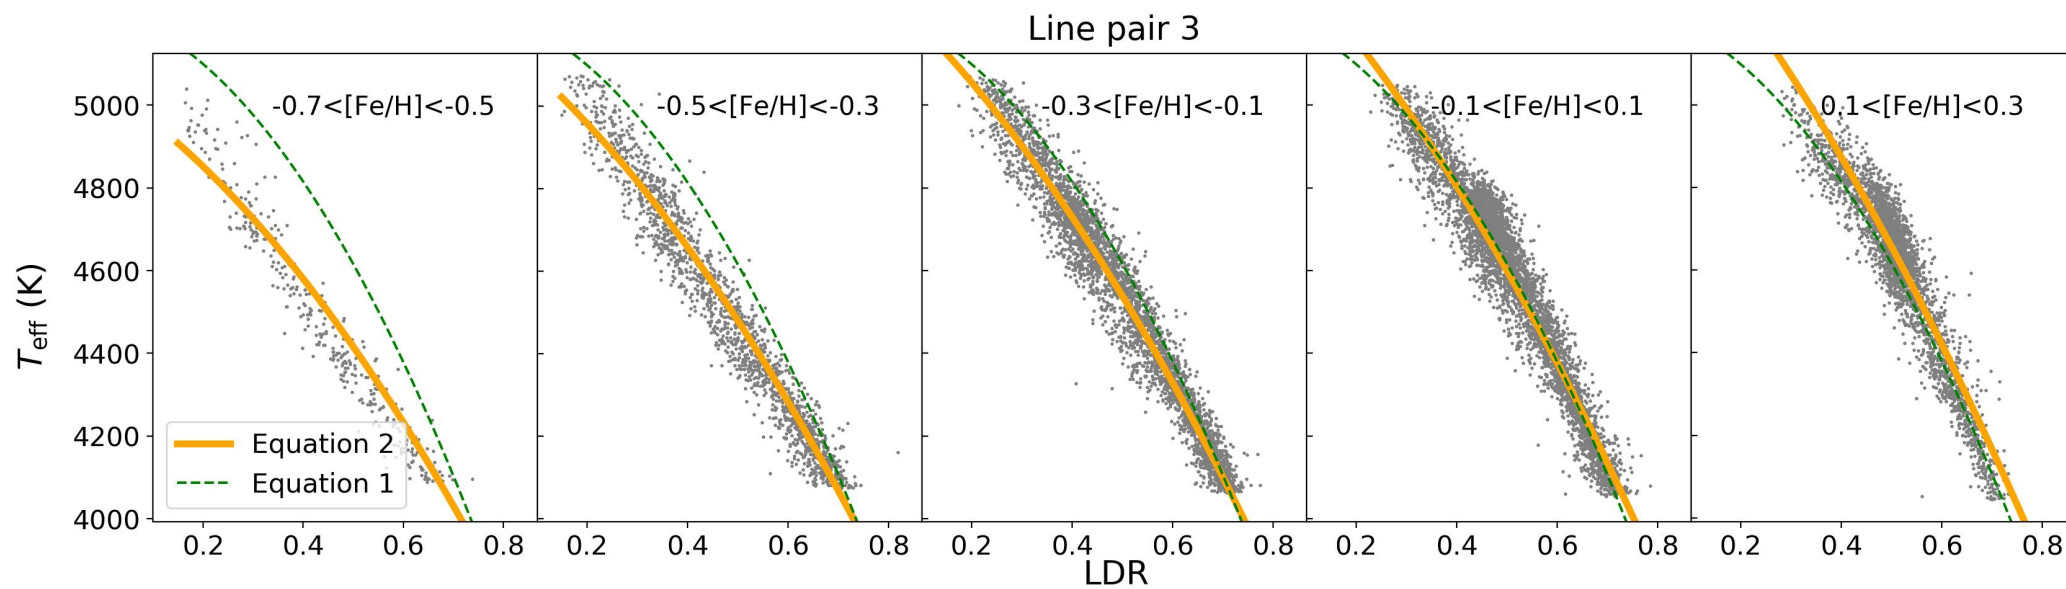

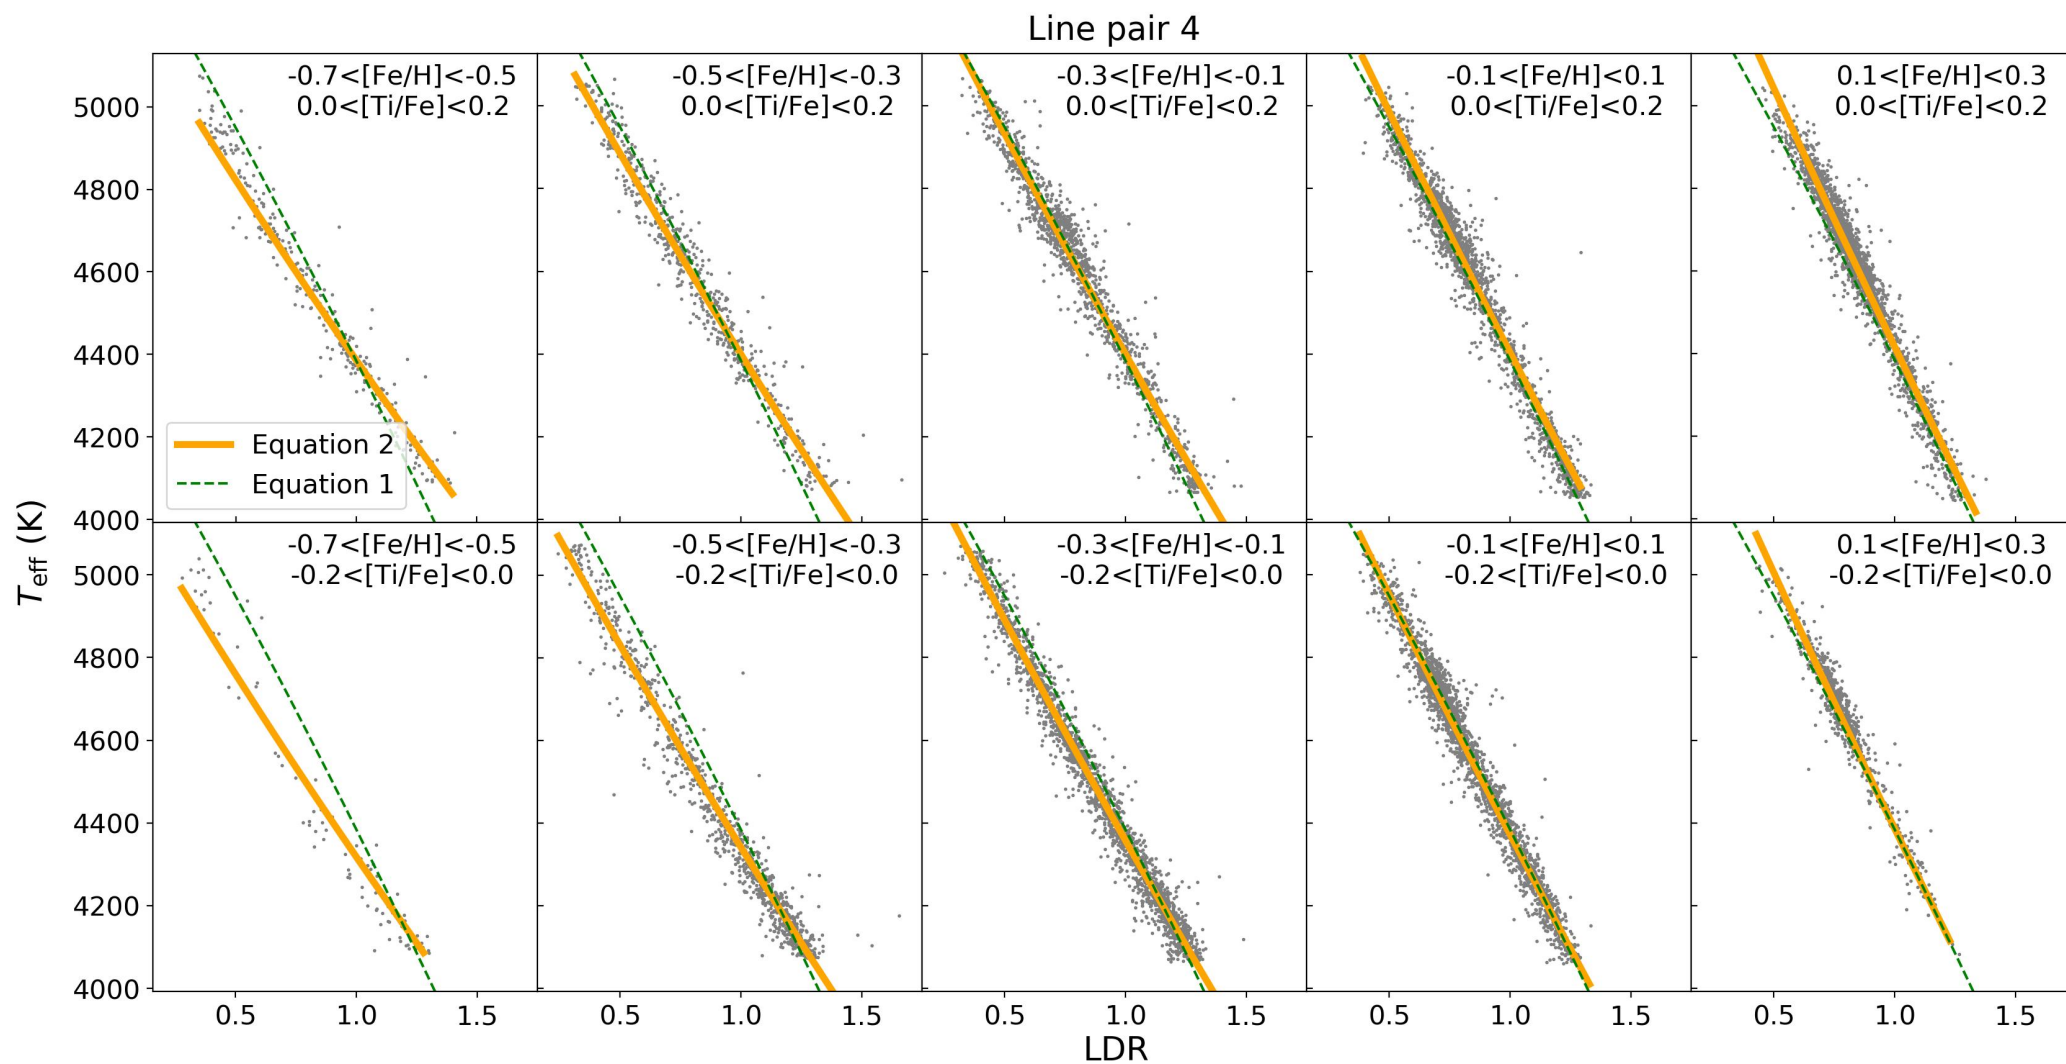

Line pair 5

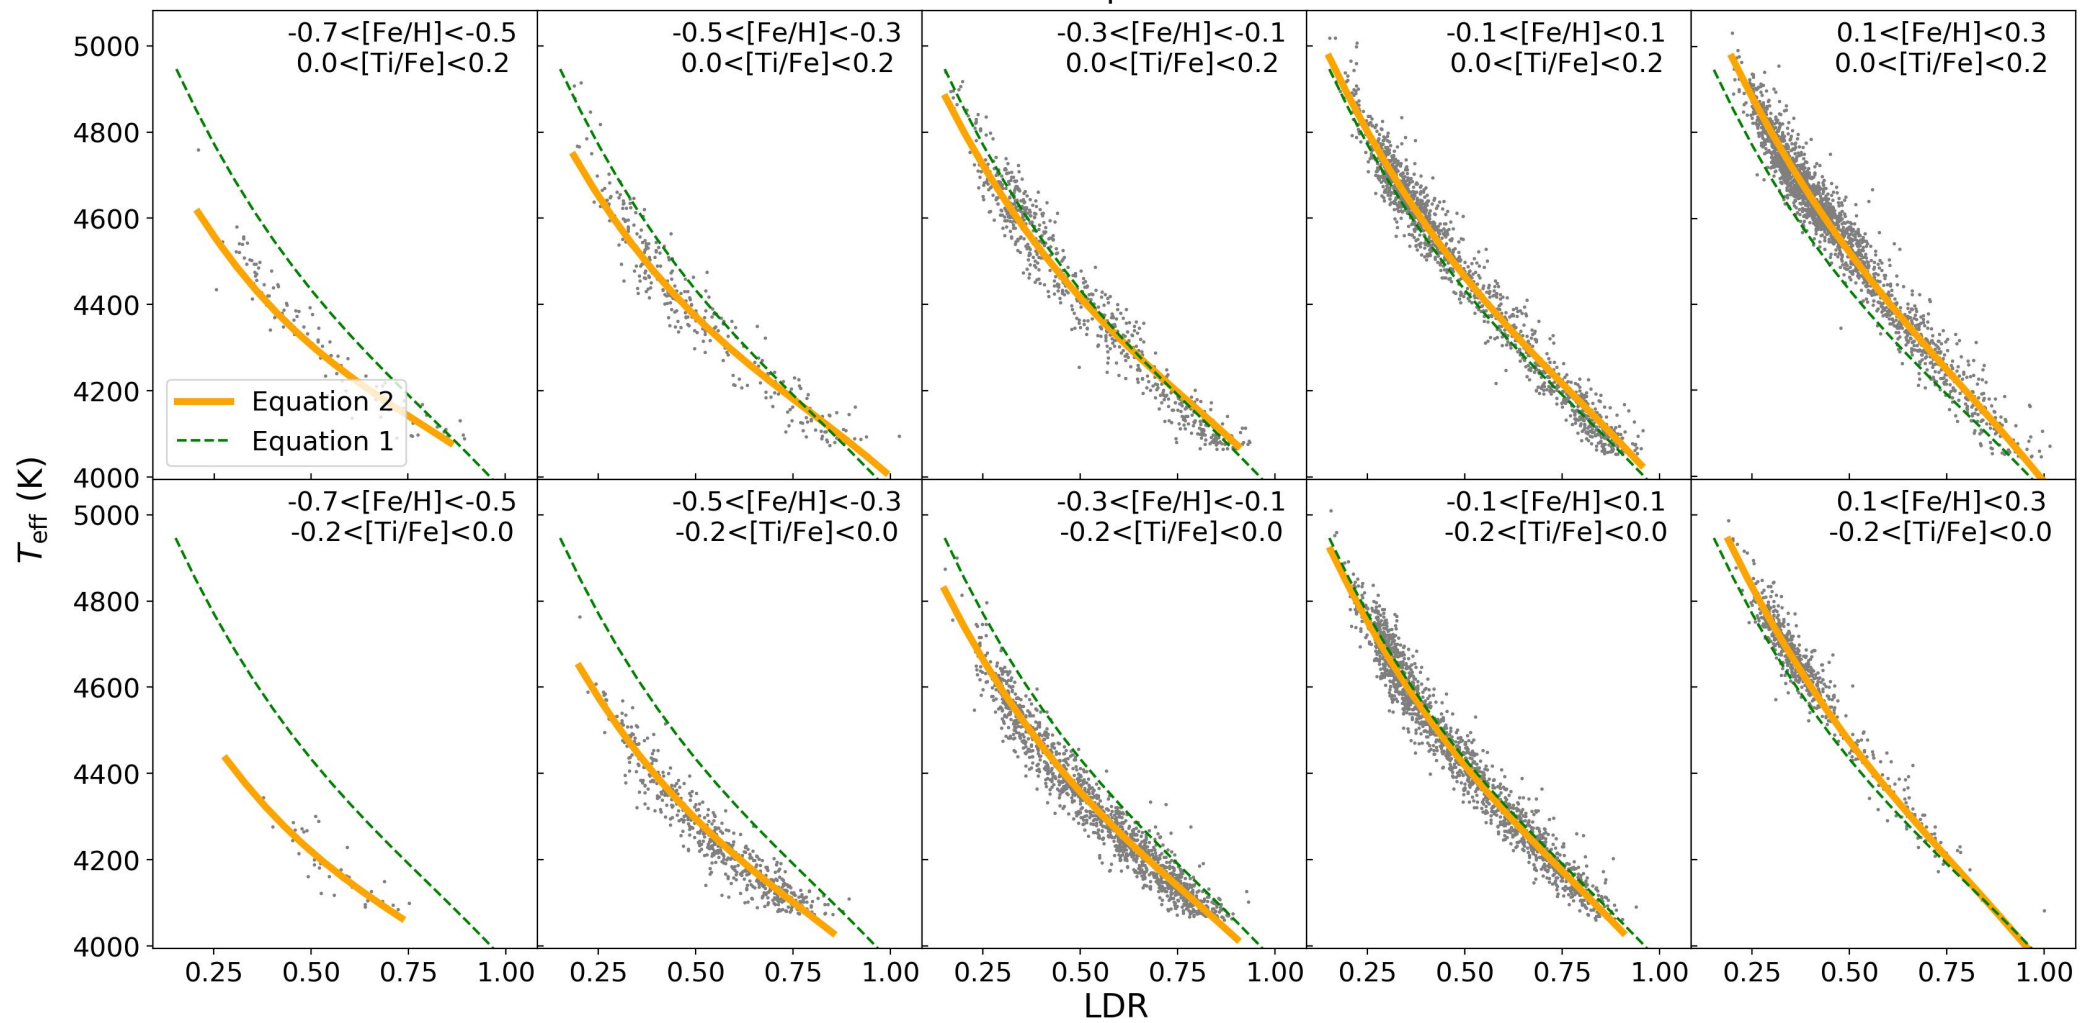

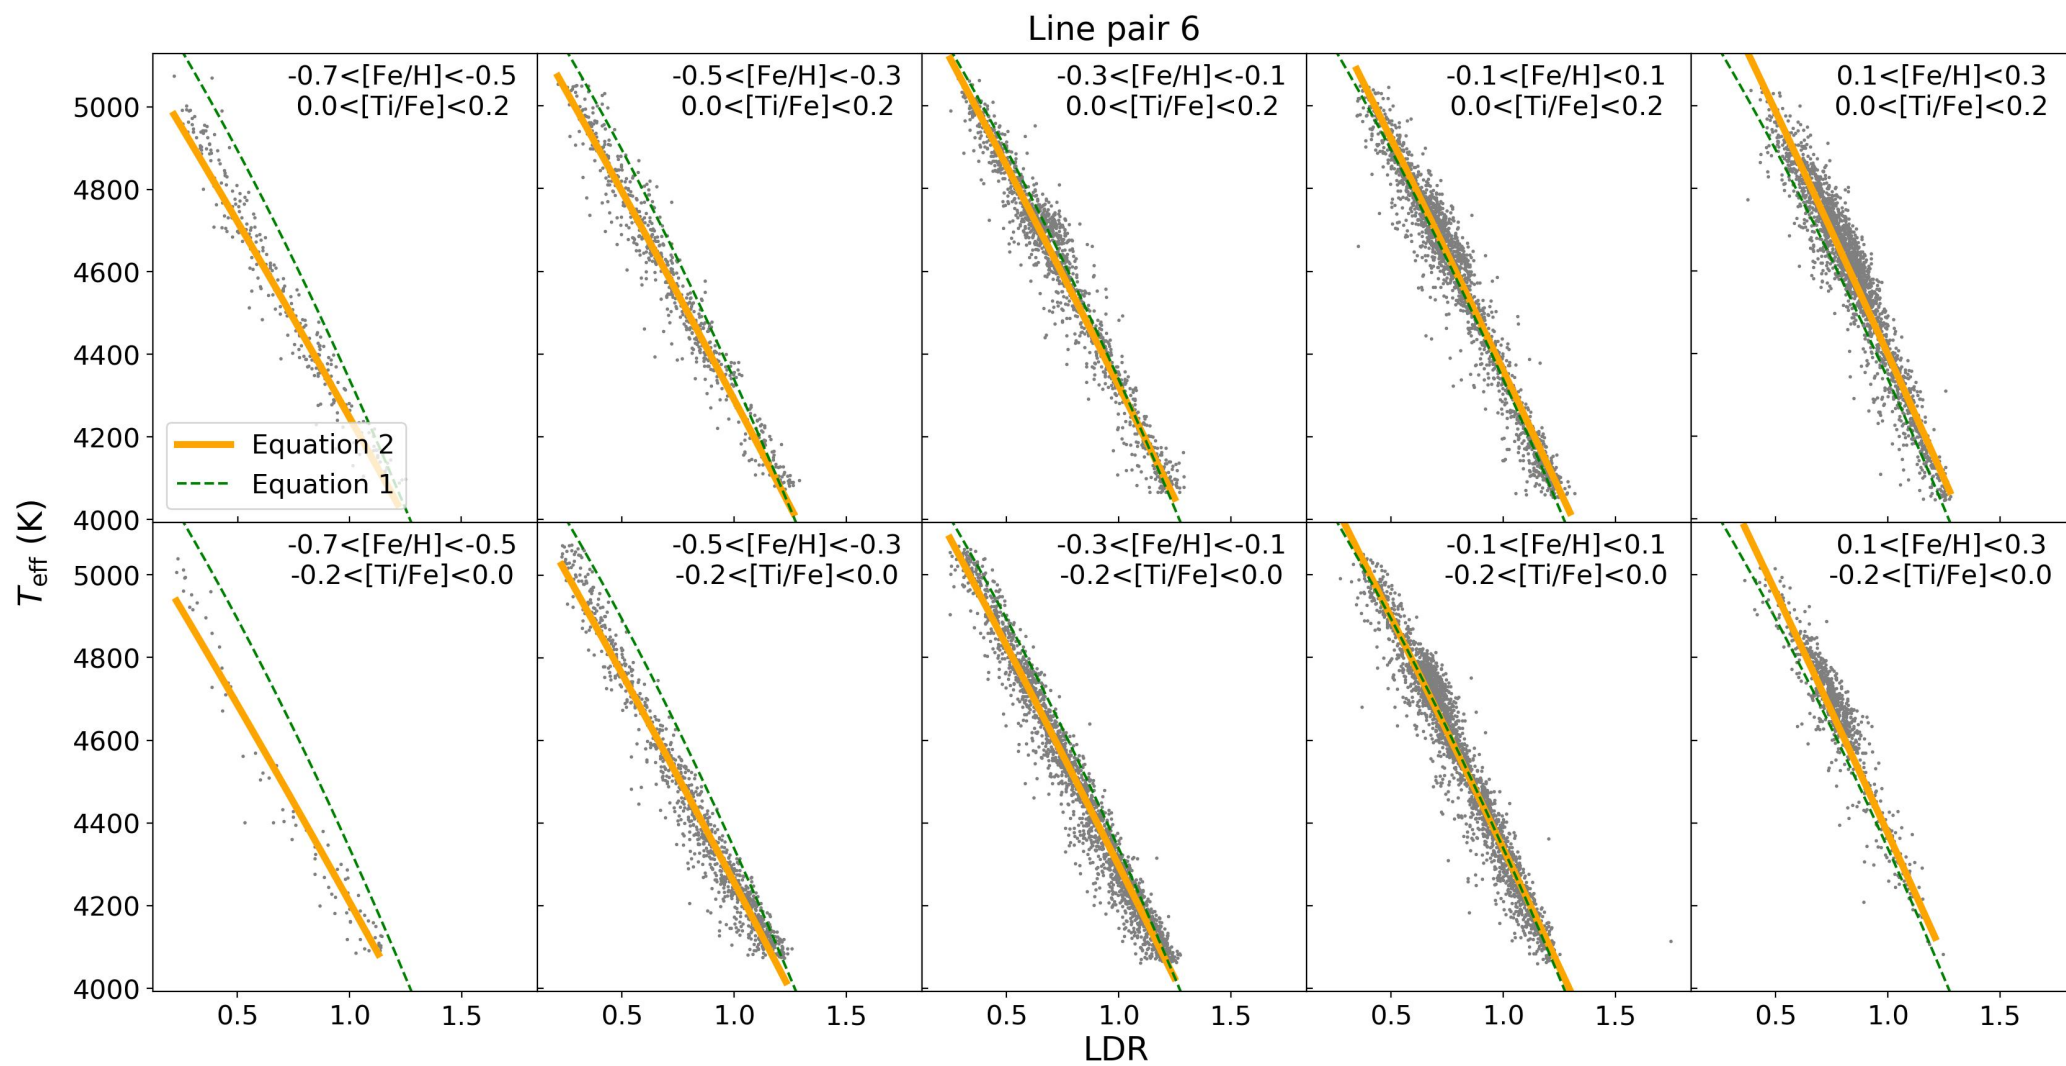

Line pair 8

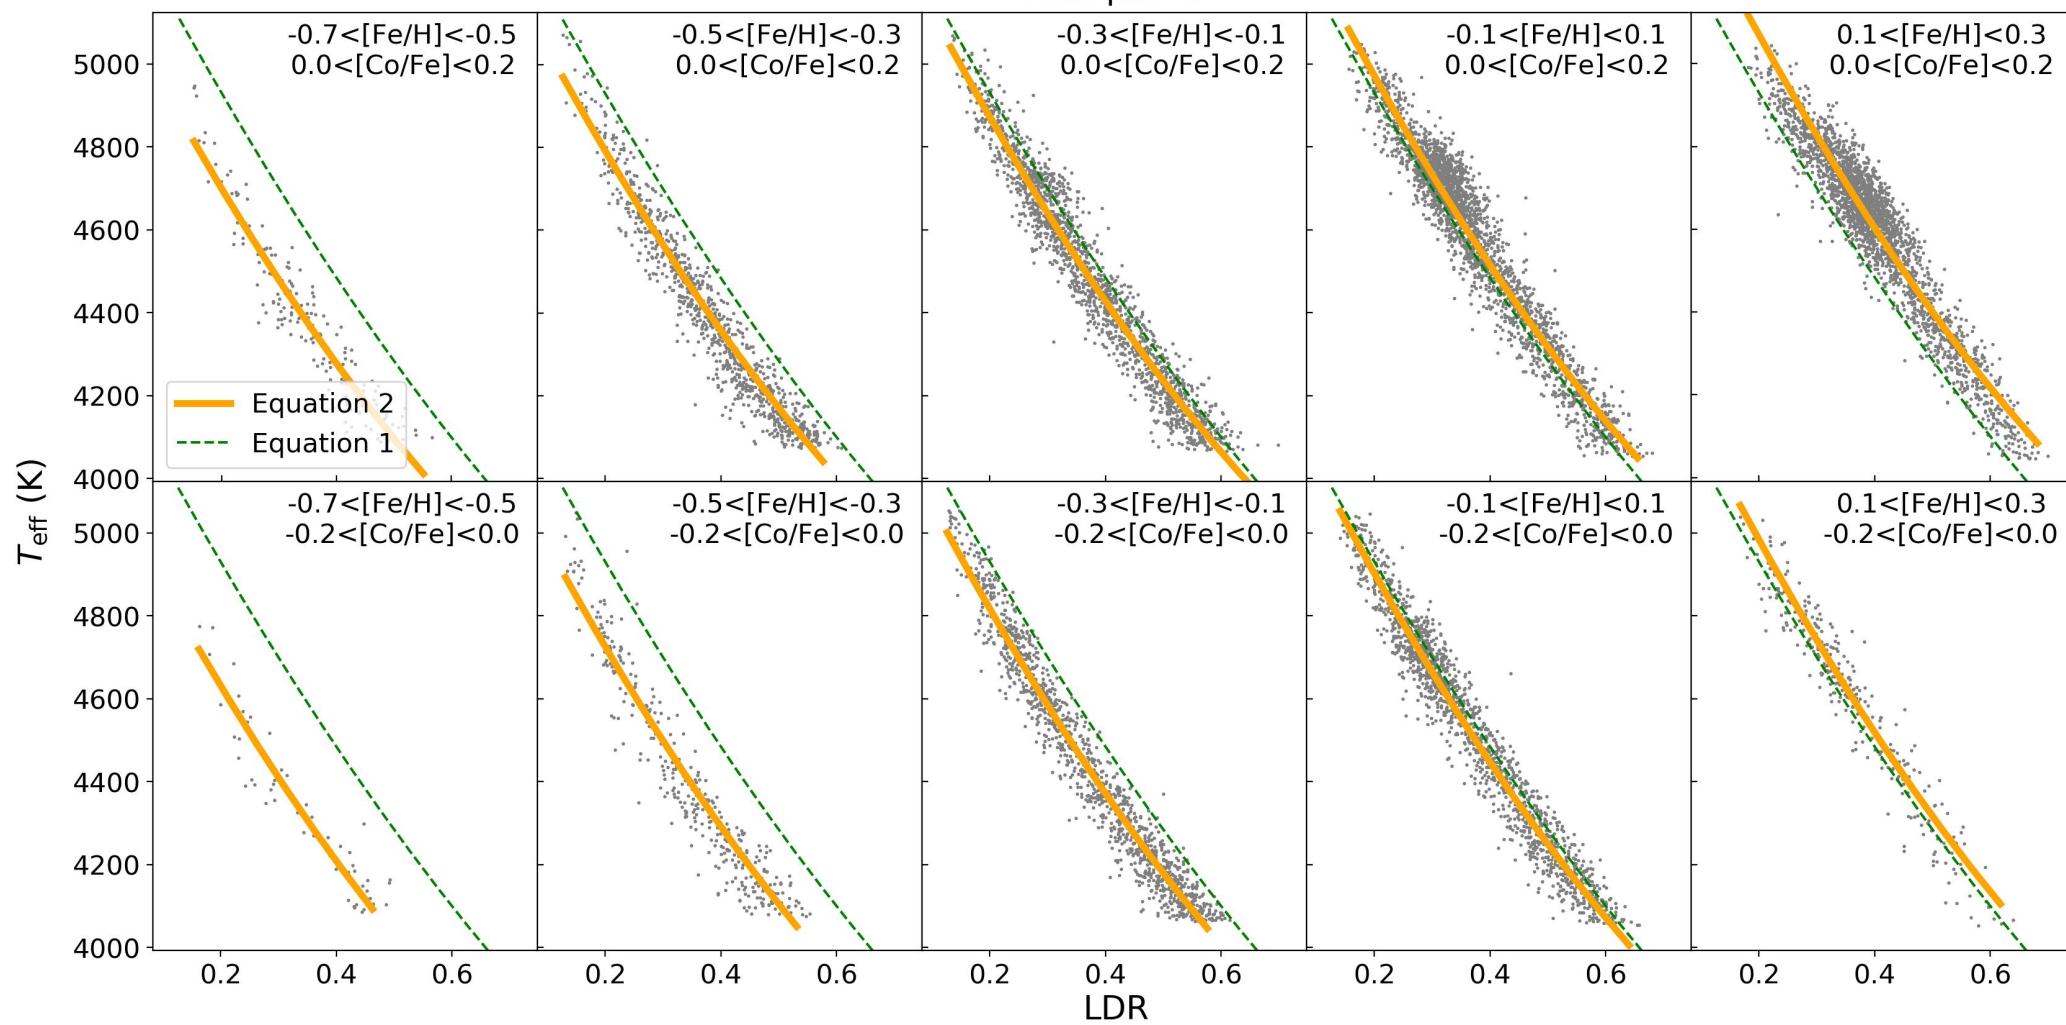

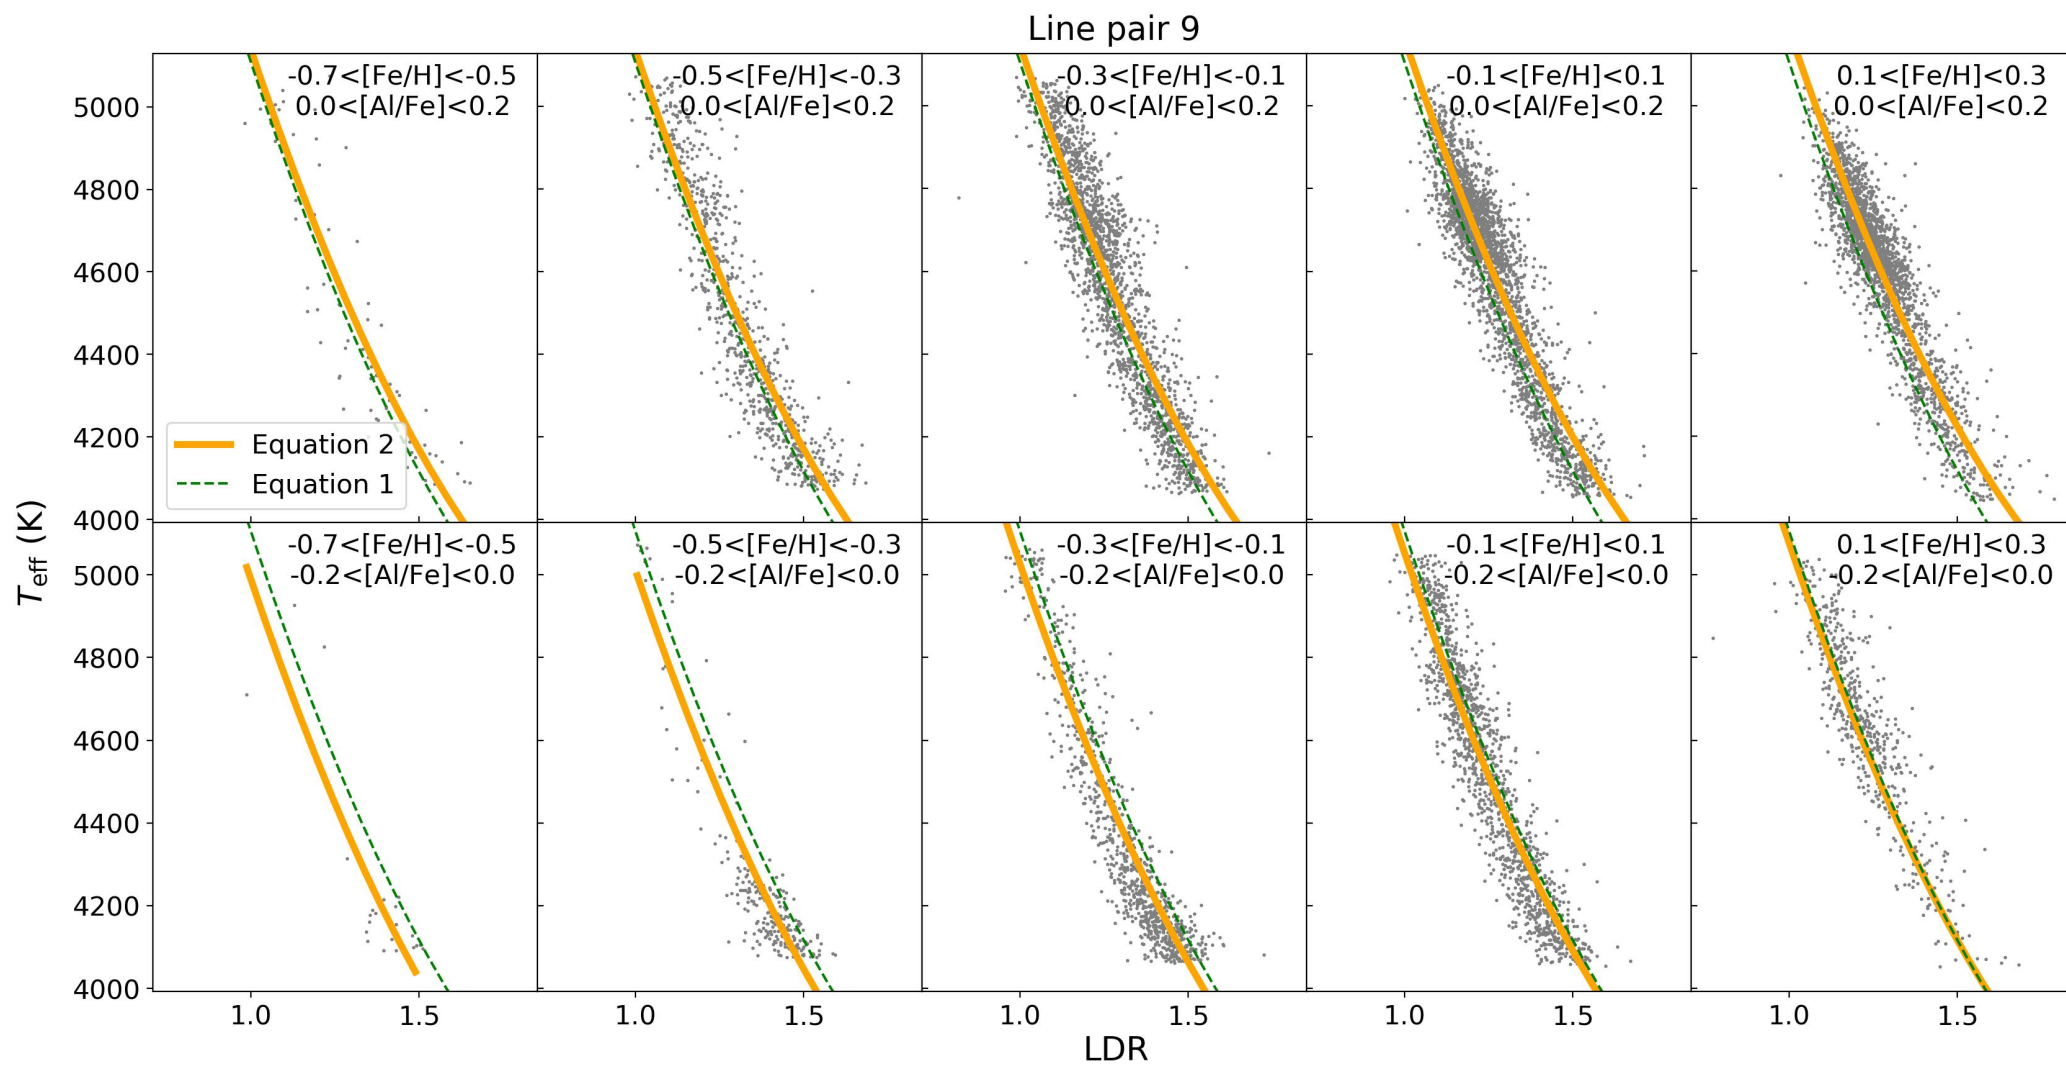

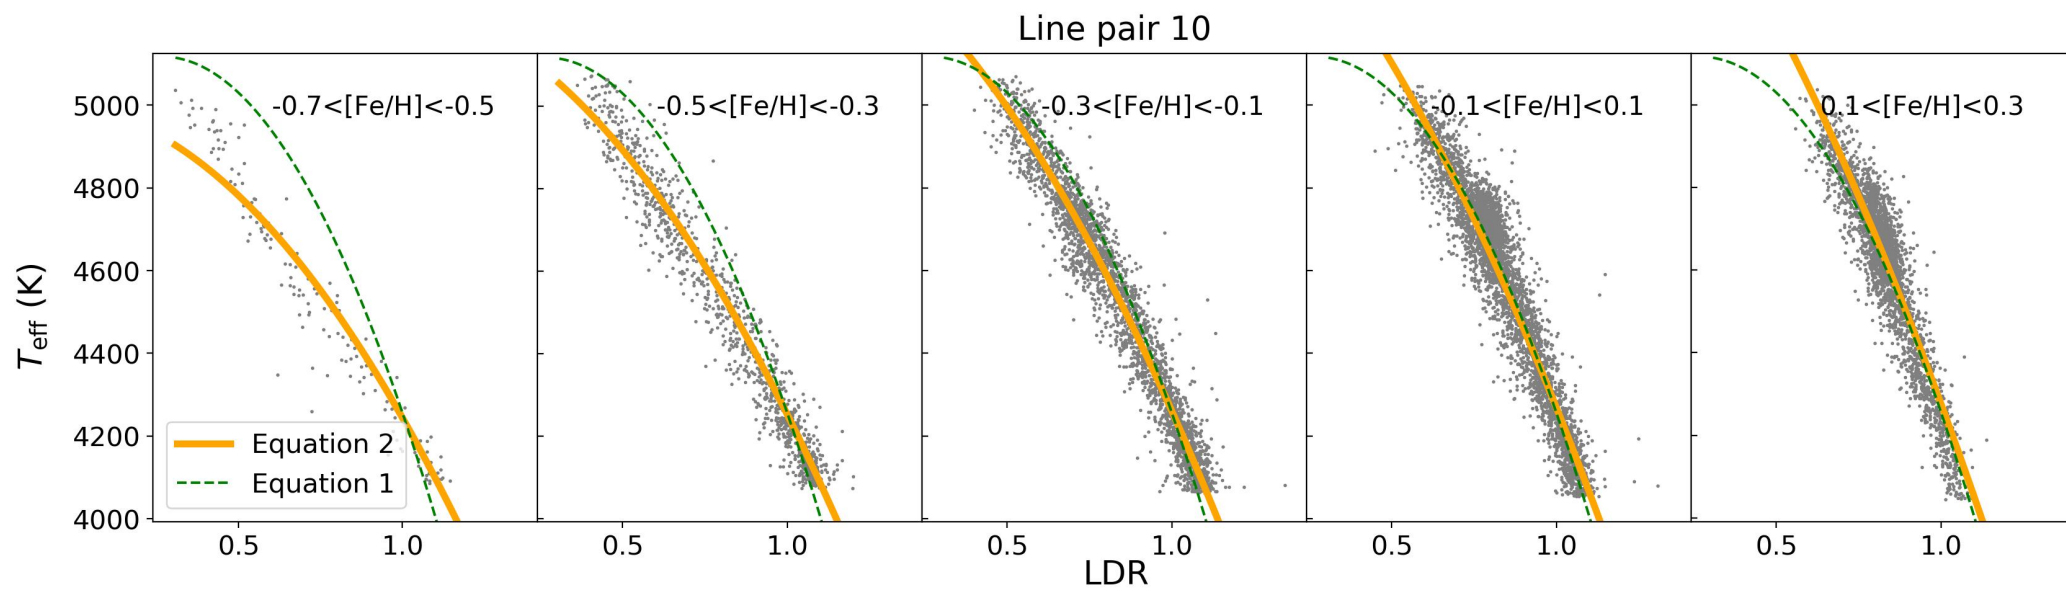

Line pair 11

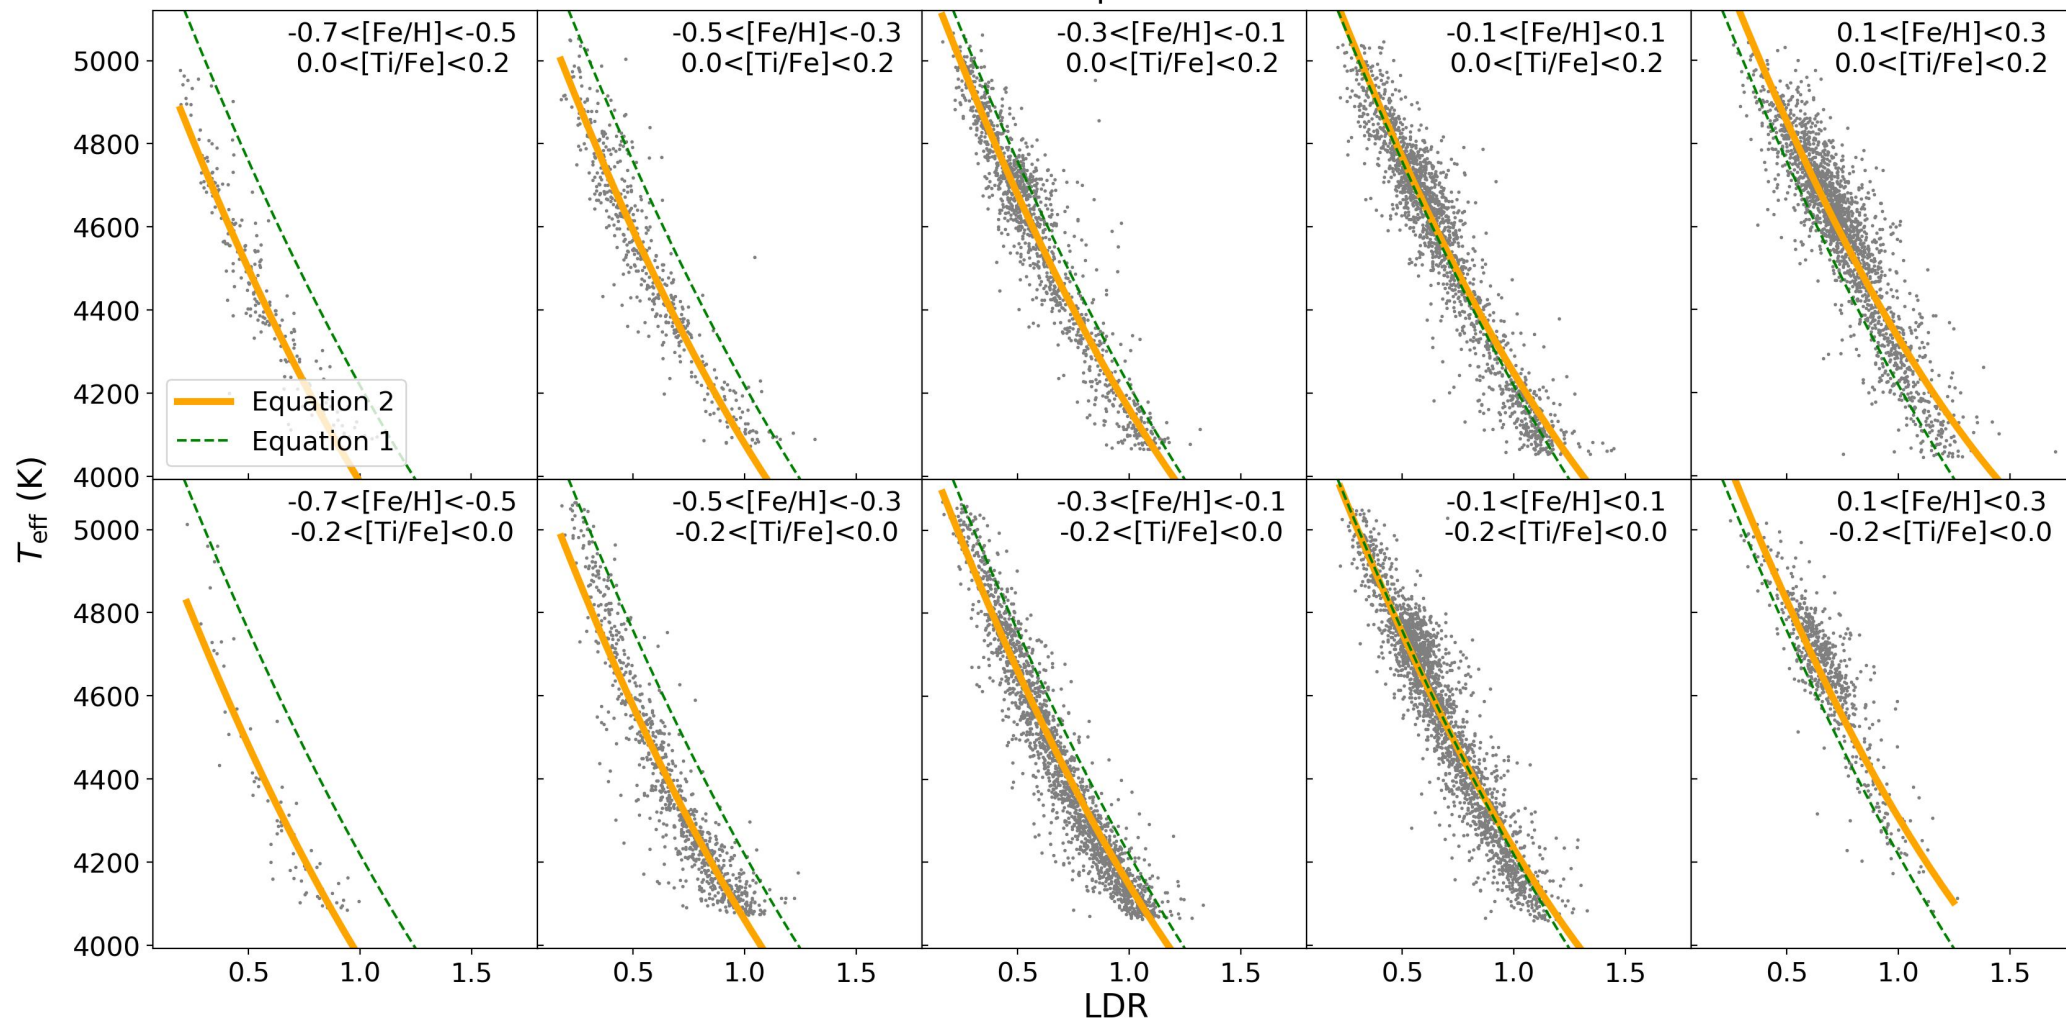

Line pair 12

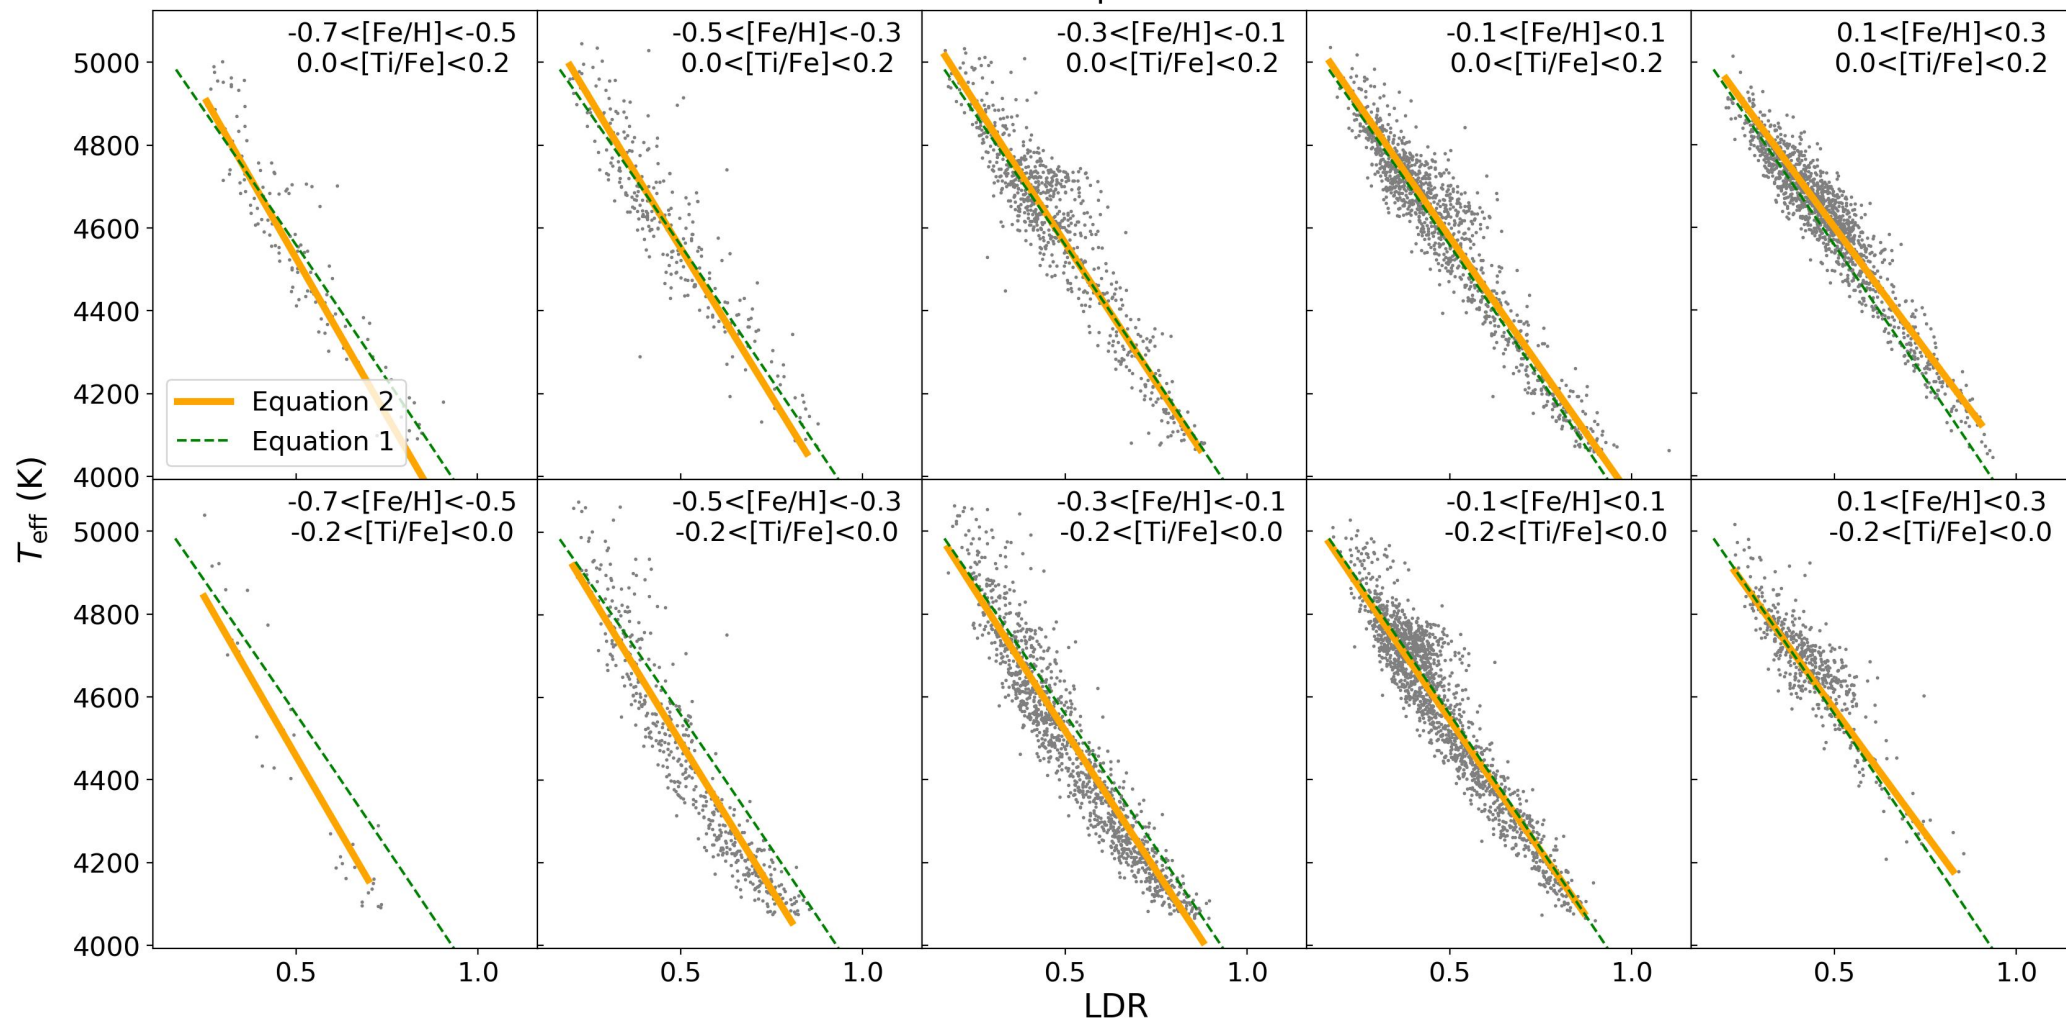

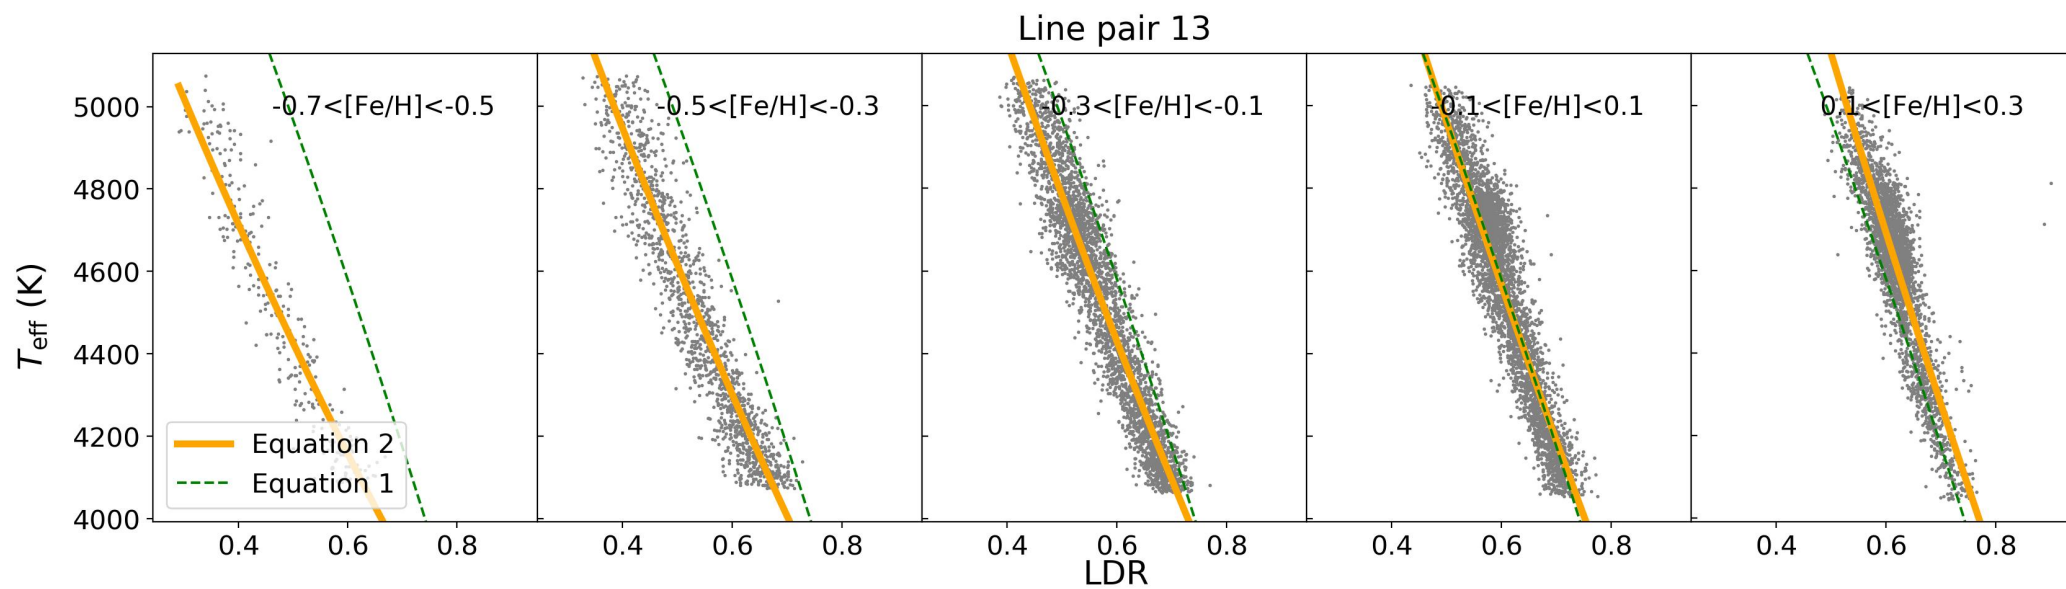

Supplement: Supplementary file 1 [file Figure4_additional_plots.pdf]
